# Supplementary material for: MedM2G: Unifying Medical Multi-Modal Generation via Cross-Guided Diffusion with Visual Invariant
Source: arXiv:2403.04290 source file (2024-03-07)
Supplement: Supplementary file 1 [file X_suppl.tex]

\clearpage
\setcounter{page}{1}
%\maketitlesupplementary
%\clearpage
%\setcounter{page}{1}
%\maketitlesupplementary
\onecolumn
The supplemental material is structured as follows:

\noindent1. We first provide a detailed introduction of the various diffusion models of the text and medical image modalities (CT, MRI, X-ray) in Appendix~\ref{sec:diffusion}.

\noindent2. We list all the pre-train tasks with corresponding datasets in Appendix~\ref{pre-train}.

\noindent3. We also give more detailed introductions of the $5$ fine-tuning tasks with $10$ datasets in Appendix~\ref{sec:fine-tuning}.

\noindent4. We then provide more details of the LDM model architecture and configuration of four medical modalities in Appendix~\ref{sec:model archi}.

\noindent5. We then conduct a more qualitative analysis of the medical report generation in Appendix~\ref{sec:medicalreport}.

\noindent6. Besides, we also conduct a comprehensive comparison between our model and the SOTA model of the medical image generation task in Appendix~\ref{sec:medicalimage}.

\noindent7. We also show more comparisons of MRI synthesis tasks in Appendix~\ref{sec:mrisys}.

\noindent8. To demonstrate the unified generation ability of medical multi-modal of our model, we provide more joint medical multi-modal generation samples in Appendix~\ref{sec:unifiedgeneration}.

\noindent9. To elucidate the effectiveness of the multi-flow training with the central alignment, we conduct more ablation studies of the multi-flow training strategy in Appendix~\ref{ablation:multi-flow}.

\noindent10. To demonstrate the innovation of our medical multi-modal generation capability, we compare detailed results of medical downstream generation tasks with current state-of-the-art general multi-modal generative models in the Appendix~\ref{comparionwithmulti}.

\noindent11. We also showcase the efficient-cost performance of our model across various training settings in Appendix~\ref{sec:computation}.

\noindent12. Lastly, we discuss the influence of different hyperparameters of the training process in Appendix~\ref{influncence}.

\section{Introduction of the Diffusion Model}
\label{sec:diffusion}
Following Versatile Diffusion~\cite{xu2023versatile}, 
we employ the widely embraced UNet~\cite{ronneberger2015unet} incorporating cross attentions as the primary architecture for our diffusion model. A portion of the UNet aligns with Stable Diffusion~\cite{rombach2022highLDM}, utilizing residual blocks for image data layers and incorporating cross-attention for contextual layers handling both text and image information.
\subsection{Text Diffusion Model}
The autoencoder of the text diffusion model is OPTIMUS~\cite{li2020optimus} with the BERT~\cite{devlin2018bert} encoder and GPT-2~\cite{radford2019languagegpt2} decoder. 
It can transform sentences bidirectionally, generating $768$-dimensional latent vectors from them, which follow a normal distribution.
For the denoising UNet module, we adopt the 1D convolution in the residual blocks~\cite{xu2023versatile}. We use both CLIP~\cite{radford2021learningclip} encoders as the prompt encoder $C_T$ and context encoder $V_T$ of the text modality.

%In the denoising UNet, 1D convolution is utilized in residual blocks instead of the 2D convolution found in image diffusion.
\subsection{Image Diffusion Model}
The diffusion models for the three medical image modalities (CT, X-ray, MRI) employ the same structure which follows the Stable Diffusion 1.5~\cite{rombach2022highLDM} and is initialized with the same weights. This way can transfer the knowledge and outstanding generation fidelity trained on extensive high-quality image datasets from Stable Diffusion~\cite{rombach2022highLDM} to our models. Same as the text diffuser, we also adopt the CLIP~\cite{radford2021learningclip} as the prompt encoder and context encoder of the CT, MRI, and X-ray modalities.

%\subsection{MRI Diffusion Model}
%\subsection{X-ray Diffusion Model}
\section{Pre-train Tasks with Datasets}
\label{pre-train}
\begin{table}[h]
	\centering
      \setlength{\tabcolsep}{4pt}
	
	\scalebox{1}{% Please add the following required packages to your document preamble:
% \usepackage{multirow}
% Please add the following required packages to your document preamble:
% \usepackage{multirow}\、
%\small
\begin{tabular}{lcc}
\hline
Tasks              & Datasets                    & Sample Numbers \\ \hline
{Text→Xray, X-ray→Text, Contrastive} & MIMIC-CXR~\cite{johnson2019mimic}                   & 227k           \\
{Text→CT, CT→Text, Contrastive}   & MedICat~\cite{DBLP:medicat}                     & 131k           \\
{CT→MRI, MRI→CT, Contrastive}    & Brain tumor MRI and CT scan~\cite{brainctmri} & 4.5k           \\ \hline
\end{tabular}}
\caption{The pre-training tasks with corresponding datasets and the training total numbers of the samples. Contrastive: the contrastive learning for alignment of the prompt encoders.}  
	\label{a_pre-train_tasks}
\end{table}

In Table~\ref{a_pre-train_tasks}, we outline the training objectives for MedM2G, encompassing tasks such as medical chest X-ray report generation, medical MRI synthesis, medical multi-modal translation, and contrastive learning for aligning prompt encoders.
Table~\ref{a_pre-train_tasks} furnishes a summary of the datasets, tasks, and sample numbers. The pre-training datasets are collected for the following domains: the medical image-text, text-Xray, Xray-CT, CT-MRI, which all follow the central alignment strategy for pre-training.

\noindent\textbf{MIMIC-CXR}
MIMIC-CXR~\cite{johnson2019mimic} is an extensive dataset containing $377,110$ chest X-rays linked to $227,827$ imaging studies. The data is collected from the Beth Israel Deaconess Medical Center. The images come with $14$ labels generated through the application of two natural language processing tools to the corresponding free-text radiology reports. We adopt the MIMIC-CXR to align the text and X-ray modalities, as well as the text→X-ray and X-ray→text generation tasks.

\noindent\textbf{MedICat}
MedICat~\cite{DBLP:medicat} is a collection of medical images presented in context, comprising $217,000$ images sourced from $131,000$ open-access biomedical papers. The dataset encompasses captions, and inline references for 74$\%$ of the figures, and includes manually annotated subfigures and subcaptions for a subset of the figures. This dataset includes CT scans with text reports, adopted for the aligning of the text and the CT modalities (Text→CT and CT→Text generation tasks).

\noindent\textbf{Brain tumor MRI and CT scan}
%\subsection{Pre-train Tasks}
Brain tumor MRI and CT scan~\cite{brainctmri} is a novel brain tumor dataset containing $4,500$ 2D MRI-CT slices. Paired for MRI and CT scans, the dataset comprises scan data from $41$ patients, with 2D slices extracted from the 3D volume. After registration, the 3D MRI and CT scans can be represented as a $237\times197\times189$ matrix. To ensure compatibility between training models and inputs, each 3D image is sliced, and $4,500$ pairs of 2D MRI-CT images are selected as the final training data. It is adopted for the alignment and generation between the CT and MRI modalities.

By adopting the multi-flow central alignment training approach, this alignment method leads to a natural and effective alignment even with limited paired data across all modalities. Significantly, it enables the implicit alignment of medical multi-modalities (CT, MRI, X-Ray) within the same space, facilitating versatile generation capabilities even in the absence of well-paired data.

%\subsection{Datasets}

\section{Fine-tuning Tasks with Datasets}
\label{sec:fine-tuning}

\begin{table}[h]
	\centering
      \setlength{\tabcolsep}{6pt}
	
	\scalebox{1}{% Please add the following required packages to your document preamble:
% \usepackage{multirow}
% Please add the following required packages to your document preamble:
% \usepackage{multirow}\、
%\small
\begin{tabular}{lccc}
\hline
\multicolumn{1}{l}{Tasks}                  & Datasets               & Modality    & Sample Numbers \\ \hline
\multirow{2}{*}{Medical Report Generation} & MIMIX-CXR~\cite{johnson2019mimic}              & Text, X-ray & 2,227           \\
                                           & IU X-ray~\cite{demner2016preparingiuxray}               & Text, X-ray & 3,955           \\ \hline
\multirow{3}{*}{Medical Image Generation}  & Chest X-ray~\cite{wang2017chestx}            & X-ray, Text & 112,120         \\
                                           & SLIVER07~\cite{heimann2009comparisonsliver}               & CT          & 4,159           \\
                                           & ACDC~\cite{bernard2018deepACDC}                   & MRI         & 1,902           \\ \hline
\multirow{2}{*}{MRI synthesis}             & BraTS 2020~\cite{brainctmri}             & MRI         & 4000             \\
                                           & IXI~\cite{IXI}                    & MRI         & 5500             \\ \hline
\multicolumn{1}{l}{MRI-CT translation}     & Gold Atlas male pelvis~\cite{nyholm2018mrpelvis} & MRI,CT      & 1350             \\ \hline
\multirow{2}{*}{Chest X-ray generation}    & MIMIC-CXR~\cite{johnson2019mimic}              & X-ray, Text & 2,227           \\
                                           & Chest X-ray~\cite{wang2017chestx}            & X-ray, Text & 108,948         \\ \hline
\end{tabular}}
\caption{The $5$ medical fine-tuning tasks with $10$ corresponding datasets, modality, and the total sample numbers. }  
	\label{fine-tuning}
\end{table}

\subsection{Medical Report Generation}
\noindent\textbf{MIMIX-CXR}
 The MIMIC-CXR dataset~\cite{johnson2019mimic}, contains a comprehensive set of X-ray images, consisting of 377,100 radiology images focused on the chest region, along with 227,835 accompanying reports from patients. Following RoentGen~\cite{chambon2022roentgen}, we adopt the official MIMIC split of the test set for the Chest X-ray generation task, which includes $2,227$ Xray-report samples. 
We employ the training subset of MIMIC-CXR for fine-tuning the medical report generation task and evaluate the test subset. The batch size for MIMIC-CXR is set to $64$ and the maximum output report length is set to $50$.

\noindent\textbf{IU X-ray}
The IU X-ray~\cite{demner2016preparingiuxray} is the pre-dominant medical dataset employed for the medical report generation task, which contains $7, 470$ chest X-ray images and $3,955$ related clinic reports from $3,955$ patients. 
Radiologists have provided annotations for MeSH in this dataset. The dataset comprises free-text radiology reports from clinical practices, encompassing multiple sections. We follow the original data split rates and set the batch size to $16$ for the IU X-ray training. We set the maximum output report length of the IU X-ray~\cite{demner2016preparingiuxray} to $45$.

\subsection{Medical Image Generation}
\noindent\textbf{Chest X-ray}
The ChestX-ray~\cite{wang2017chestx} dataset consists of $112,120$ chest X-ray images in PNG format, each with a resolution of $1024 \times 1024$ pixels. We follow the original data splits of $70\%/10\%/20\%$ train/val/test for the medical image generation tasks.

\noindent\textbf{SLIVER07}
For the SLIVER07~\cite{heimann2009comparisonsliver}dataset, we utilized 20 scans available in the training dataset. Each slice was converted to a PNG image without any additional preprocessing. The dataset comprises a total of $4,159$ images, each with a resolution of $512\times512$ pixels.

\noindent\textbf{ACDC}
The ACDC~\cite{bernard2018deepACDC} dataset consists of 150 cardiac cine-magnetic resonance imaging (MRI) exams. We utilized the training dataset, which includes 100 exams. The images were rescaled to the range $[0, 255]$ using SimpleITK and zero-padded. Each slice was then converted into a 2D PNG image. In total, this dataset comprises $1,902$ images, each with a resolution of $512 \times 512$ pixels.

We all follow the original fine-tuning settings which undergoes end-to-end training with Adam using standard parameters ($\beta_1$ = 0.9 and $\beta_2$ = 0.999). Training occurs in mini-batches of size $16$, with an initial learning rate set at $0.001$. The learning rate is decayed by a factor of $10$ whenever the validation loss reaches a plateau after an epoch. 

\subsection{MRI Synthesis Task}
\noindent\textbf{BraTS}
The BraTS~\cite{brainctmri} dataset analyzed T1, T2, and Fluid Attenuated Inversion Recovery (FLAIR) weighted brain MR images from 55 patients with gliomas, partitioned into training, validation, and test sets with 25, 10, and 20 subjects, respectively. The T2 and FLAIR volumes were registered to the T1 volume in the validation/test set. For each subject, 100 axial cross-sectional slices containing brain tissue were selected. Different scanning protocols were employed by multiple institutions.

\noindent\textbf{IXI}
The IXI~\cite{IXI} dataset analyzed T1, T2, and Proton Density (PD) weighted images from 40 healthy subjects, with $(25, 5, 10)$ individuals retained for (training, validation, testing). T2 and PD volumes were registered to the T1 volume in the validation/test set. For each subject, 100 axial cross-sectional slices containing brain tissue were selected. The scanning parameters for T1 were TE=$4.6ms$, TR=$9.81ms$, for T2, TE=$100ms$, TR=$8178.34ms$, and for PD images, TE=$8ms$, TR=$8178.34ms$. The common spatial resolution was $0.94\times0.94\times1.2$${mm}^3$.

The batch size is set to $8$, and the learning rate is set to $9.6e-5$. Noise variances, ranging from $\beta_1$ = $10e-4$ to $\beta_T$ = $0.02$, are employed.

\subsection{MRI-CT Translation}
\noindent\textbf{Gold Atlas male pelvis}
The pelvic~\cite{nyholm2018mrpelvis} dataset analyzed T1 and T2-weighted MRI as well as CT images of 15 subjects, divided into $(9, 2, 4)$ individuals for (training, validation, testing). T1 and CT volumes were registered to the T2 volume in the validation/test set. For each subject, 90 axial cross-sectional slices were selected. For T1 scans, specifications included TE=$7.2ms$, TR=$500-600ms$, with a resolution of $0.88\times0.88\times3$${mm}^3$, or TE=$4.77ms$, TR=$7.46ms$, with a resolution of $1.10\times1.10\times2$${mm}^3$. For T2 scans, specifications included TE=$97$ms, TR=$6000$-$6600$ms, with a resolution of $0.88\times0.88\times2.50$${mm}^3$, or TE=$91$-$102$ms, TR=$12000$-$16000$ms, with a resolution of $0.88-1.10\times0.88-1.10\times2.50$${mm}^3$. For CT scans, specifications included a resolution of $0.10\times0.10\times3$${mm}^3$ with Kernel=B30f or a resolution of $0.10\times0.10\times2$${mm}^3$ with Kernel=FC17. To accelerate the synthesis task for MRI scans, $4\times$ retrospective undersampling was performed on fully sampled MRI data in 2D to obtain low-resolution images with a $16x$ acceleration rate. The training batch size is set to $64$.

\subsection{Chest X-ray Generation Task}

\noindent\textbf{MIMIC-CXR}
We assess the quality and clinical effectiveness of the generated chest X-rays and reports across various dimensions. Standard evaluation metrics for generative models, including FID and BLEU, are employed. A total of 208,534 studies, each containing a maximum of 3 chest X-rays with common views (PA, AP, and LATERAL3), are selected for evaluation. The dataset follows the official split of MIMIC-CXR (training set: 204,102, validation set: 1,659, test set: 2,773).

\noindent\textbf{Chest X-ray}
The ChestX-ray~\cite{wang2017chestx} includes $108,948$ frontal-view X-ray images belonging to 32,717 distinct patients. The dataset is annotated with eight disease labels extracted from radiological reports using natural language processing. Each image can have multiple labels. We follow the original data splits of $70\%/10\%/20\%$ train/val/test for the chest X-ray generation task.
The batch size is set to $16$ with an initial learning rate of $0.001$. We adopt other Adam optimizer with $\beta_1$ = $0.9$ and $\beta_2$ = $0.999$.
%All of us adhere to the initial fine-tuning configurations, engaging in end-to-end training with Adam and employing standard parameters ($\beta_1$ = 0.9 and $\beta_2$ = 0.999). Training is conducted in mini-batches, each comprising 16 samples, and begins with an initial learning rate of 0.001.

\section{Model Architecture and Configuration}
\label{sec:model archi}
We provide more details of the model architecture and configuration in Table~\ref{architecture}. Following CoDi~\cite{tang2023codi}, the diffusion models of four modalities (Text, CT, MRI, X-ray) are all based on the UNet structure with specific settings.
The $\lambda_1$ in Eq. 4 is set to $5e-3$. The experiment for the influence of $\lambda_1$  is conducted in Appendix~\ref{influncence}.

%\section{Fine-tuning Tasks with Datasets}
\begin{table}[h]
	\centering
      \setlength{\tabcolsep}{6pt}
	
	\scalebox{1}{% Please add the following required packages to your document preamble:
% \usepackage{multirow}
% Please add the following required packages to your document preamble:
% \usepackage{multirow}\、
\small
\begin{tabular}{lllll}
\hline
Modality                & Text LDM            & X-ray LDM & CT LDM            & MRI LDM           \\ \hline
\textbf{Hyperparameter}          &                     &           &                   &                   \\
Architecture            & LDM                 & LDM       & LDM               & LDM               \\
z-shape                 & 768 ×1×1            & 4×64×64   & 4×64×64           & 4×64×64           \\
Channels                & 320                 & 320       & 320               & 320               \\
Depth                   & 2                   & 4         & 4                 & 4                 \\
Channel multiplier      & 1,2,4,4             & 1,2,4,4   & 1,2,4,4           & 1,2,4,4           \\
Attention resolutions   & 64,32,16            & 64,32,16  & 64,32,16          & 64,32,16          \\
Head channels           & 32                  & 32        & 32                & 32                \\
Number of heads         & 8                   & 8         & 8                 & 8                 \\
CA embed dim            & 768                 & 768       & 768               & 768               \\
Embedding Layer dim            & 768                 & 768       & 768               & 768               \\
CA resolutions          & 64,32,16            & 64,32,16  & 64,32,16          & 64,32,16          \\
Autoencoders            & Optimus             & AutoKL    & AutoKL            & AutoKL            \\
Weight initialization   & Versatile Diffusion & SD-1.5    & SD-1.5            & SD-1.5            \\
Parameterization        &  $\epsilon$                   &    $\epsilon$         & $\epsilon$                    &     $\epsilon$                \\
Learning rate           & 5.e-05            & 2e-05  & {1e-06} & {1e-06} \\
Total batch size        & 1024                & 256       & 128               & 128               \\ \hline
\textbf{Diffusion Setup}         &                     &           &                   &                   \\
Diffusion steps         & 1000                & 1000      & 1000              & 1000              \\
Noise schedule          & Linear              & Linear    & Linear            & Linear            \\
$\beta_0$ & 0.00085             & 0.00085   & 0.00085           & 0.00085           \\
$\beta_T$ & 0.012               & 0.012     & 0.012             & 0.012             \\ \hline
\textbf{Sampling Parameters}     &                     &           &                   &                   \\
Sampler                 & DDIM                & DDIM      & DDIM              & DDIM              \\
Steps                   & 50                  & 50        & 50                & 50                \\
$\eta$     & 1.0                 & 1.0       & 1.0               & 1.0               \\
Guidance scale          & 2.0                 & 2.0       & 2.0               & 2.0               \\ \hline
\end{tabular}}
\caption{The architecture and configuration of different diffusion models. SD: Stable Diffusion. CA: Cross-attention layer. Embedding Layer: the embedding layer $\mathbb{F}_{emb}$.}  
	\label{architecture}
\end{table}

%\noindent\textbf{Medical Report Generation}

%\noindent\textbf{Medical Image generation}

%\textbf{}\noindent\textbf{MRI Sysnethsis}

%\noindent\textbf{MRI-CT Translation}

%\noindent\textbf{Chest X-ray Generation}

\section{Qualitative Analysis of Medical Report Generation}
\label{sec:medicalreport}
\begin{figure*}[h]
\centering
\includegraphics[width=1\linewidth]{a_g.pdf}
\caption{More case studies of medical report generation task between ours with SOTA model.}
\label{a_g}
\end{figure*}
We conduct a more qualitative analysis of the medical report generation task in Fig.~\ref{a_g}.
By comparison of our model with the SOTA model Kuit~\cite{huang2023kiut} in Fig.~\ref{a_g}, our model excels in producing more precise and semantically rich reports. The majority of MeSH terms are accurately forecasted, as highlighted in green.

\section{More Comparison of Medical Text-Image Generation}
\label{sec:medicalimage}
\begin{figure*}[h]
\centering
\includegraphics[width=1\linewidth]{a_ig.pdf}
\caption{More case studies of medical image generation task between ours with SOTA model.}
\label{a_ig}
\end{figure*}
Through a comprehensive comparison with state-of-the-art models GLIGEN~\cite{li2023gligen} in Fig.~\ref{a_ig}, our model stands out in its capacity to intricately and semantically generate descriptions of crucial pathological regions, as outlined in input medical reports, particularly evident in detailing small nodules.

\section{More Comparison of MRI systhesis}
\label{sec:mrisys}
\begin{figure*}[h]
\centering
\includegraphics[width=1\linewidth]{a_mri2.pdf}
\caption{More comparisons of MRI synthesis task (T1→T2, T1→PD) between ours with SOTA model CoLa-Diff.}
\label{a_mri}
\end{figure*}

\begin{table*}
	\centering
	%\resizebox{8cm}{
	\scalebox{1}{% Please add the following required packages to your document preamble:
% \usepackage{multirow}
% Please add the following required packages to your document preamble:
% \usepackage{multirow}\
\small
	\setlength{\tabcolsep}{12pt}
	
%\begin{tabular}{lcccccccccccc}
\begin{tabular}{ccccccc}
\hline
\multirow{3}{*}{Methods} & \multicolumn{4}{c}{BRATS}                                              & \multicolumn{2}{c}{IXI}         \\ \cline{2-7} 
                         & \multicolumn{2}{c}{T2+T1+FLAIR→T1ce} & \multicolumn{2}{c}{T2+T1ce+T1→FLAIR} & \multicolumn{2}{c}{T2+T1→PD}    \\ \cline{2-7} 
                         & PSNR              & SSIM             & PSNR              & SSIM             & PSNR           & SSIM           \\ \hline
MM-GAN~\cite{sharma2019missingmmgan}                   & 26.30$_{\pm 1.91}$              & 91.22$_{\pm 2.08}$            & 24.09$_{\pm 2.14}$            & 88.32$_{\pm 1.98}$   & 30.61$_{\pm 1.25}$          & 95.42$_{\pm 1.78}$    \\
Hi-Net~\cite{zhou2020hinet}                   & 27.02$_{\pm 1.26}$             & 93.35$_{\pm 1.34}$            & 25.87$_{\pm 2.82}$             & 91.22$_{\pm 2.13}$            & 31.79$_{\pm 1.66}$          & 96.51$_{\pm 2.23}$          \\
ProvoGAN~\cite{yurt2022progressivelyProvoGAN}                  & 29.26$_{\pm 2.50}$             & 93.96$_{\pm 2.34}$            & 25.64$_{\pm 2.77}$             & 90.42$_{\pm 3.13}$                  & 29.93$_{\pm 2.13}$          & 94.62$_{\pm 2.46}$          \\
LDM~\cite{rombach2022highLDM}                    & 25.61$_{\pm 2.48}$          & 89.18$_{\pm 2.55}$            & 23.12$_{\pm 3.16}$             & 86.90$_{\pm 3.24}$         & 27.36$_{\pm 1.96}$          & 91.52$_{\pm 2.16}$          \\
CoLa-Diff~\cite{jiang2023cola}            & 29.35$_{\pm 2.40}$             & 94.18$_{\pm 2.46}$            & 26.68$_{\pm 2.74}$             & 91.89$_{\pm 3.11}$       & 32.24$_{\pm 1.86}$          & 96.95$_{\pm 2.61}$          \\ \hline
\textbf{ours}             & \textbf{30.12$_{\pm 1.78}$}    & \textbf{95.32$_{\pm 2.64}$}   & \textbf{27.89$_{\pm 2.84}$}    & \textbf{93.01$_{\pm 1.68}$}   & \textbf{34.12$_{\pm 1.82}$} & \textbf{97.88$_{\pm 2.82}$} \\ \hline
\end{tabular}}
\caption{The comparisons between our model MedM2G and advanced MRI synthesis models on BRATS and IXI datasets. } 
	\label{mrisynthesis}
\end{table*}

More comparisons of MRI synthesis tasks (T1→T2, PD→T1) are listed in Table~\ref{mrisynthesis} and Fig.~\ref{a_mri}. Detailed comparative experiments demonstrate that our model excels in generating intricate brain sulci and tumor boundaries, effectively preserving anatomical structure.

\section{More Samples of Unified Multi-modality Joint Generation}
\label{sec:unifiedgeneration}
\begin{figure*}[h]
\centering
\includegraphics[width=1\linewidth]{a_unified2.pdf}
\caption{More generation samples of unified multi-modal joint generation task (X-ray, MRI, CT).}
\label{a_unified}
\end{figure*}
We conduct more samples of unified multi-modal joint generation tasks in Fig.~\ref{a_unified}. Our model achieves a unified generation of medical images in three modalities (CT, MRI, X-ray) and implicitly integrates various medical modalities to compose semantic clinical information in a unified manner.

\section{Ablation Study of Multi-flow Training Strategy}
\label{ablation:multi-flow}
We conduct more ablation studies of multi-flow training in Table ~\ref{abalation_data}. It can be observed that models pre-trained on MIMIC-CXR~\cite{johnson2019mimic} achieve a significant improvement in medical image-text generation tasks. Additionally, with the incorporation of the MedICat~\cite{DBLP:medicat} pre-training dataset, accompanied by efficient-cost computational resources, the results of $5$ generation tasks, including X-ray, MRI, and CT, have seen further enhancement. Furthermore, the inclusion of paired MRI-CT data has advanced the performance of unified generation across modalities, accompanied by a modest increase in computational resources.

\begin{table*}[h]
	\centering
	%\resizebox{8cm}{
	\scalebox{0.82}{% Please add the following required packages to your document preamble:
% \usepackage{multirow}
% Please add the following required packages to your document preamble:
% \usepackage{multirow}\
\small
	\setlength{\tabcolsep}{1pt}
	
%\begin{tabular}{lcccccccccccc}
\begin{tabular}{lccccccccccc}
\hline
\multicolumn{1}{c}{\multirow{2}{*}{\begin{tabular}[c]{@{}c@{}}Pre-train\\ Dataset\end{tabular}}} & \multicolumn{3}{c}{MIMIC-CXR}                    & ACDC           & \begin{tabular}[c]{@{}c@{}}MIMIC-CXR\\ (X-Ray generation)\end{tabular} & \multicolumn{2}{c}{\begin{tabular}[c]{@{}c@{}}BraTS2020\\ (T2+T1→PD)\end{tabular}} & \multicolumn{2}{c}{\begin{tabular}[c]{@{}c@{}}Pelvic\\ T2→CT\end{tabular}} & \begin{tabular}[c]{@{}l@{}}Pre-training\\  time\\ /epoch\end{tabular} & \begin{tabular}[c]{@{}l@{}}Add\\ Parameter\end{tabular} \\ \cline{2-12} 
\multicolumn{1}{c}{}                                                                             & BLEU-1         & BLEU-4         & ROUGE\_L       & Fid(↓)         & Fid(↓)                                                                 & PSNR                                     & SSIM                                    & PSNR                                 & SSIM                                & /h                                                                    & /M                                                      \\ \hline
MIMIC                                                                                            & 0.389$_{\pm 0.009}$          & 0.129$_{\pm 0.011}$          & 0.283$_{\pm 0.012}$          & 20.13          & 3.1                                                                    & 33.76$_{\pm 2.12}$                                    & 97.41$_{\pm 1.87}$                                   & 27.22$_{\pm 0.23}$                                & 88.68$_{\pm 1.49}$                               & 0.7                                                                   & 46.4                                                    \\
MIMIC+MedICat                                                                                    & 0.399$_{\pm 0.008}$          & 0.136$_{\pm 0.012}$          & 0.298$_{\pm 0.011}$          & 16.68          & 2.2                                                                    & 33.98$_{\pm 1.68}$                                    & 97.67$_{\pm 1.72}$                                   & 27.38$_{\pm 0.37}$                                & 88.99$_{\pm 1.47}$                               & 1.4                                                                   & 85.3                                                    \\
\textbf{MIMIC+MedICat+MRI-CT}                                                          &  \multicolumn{1}{c}{\textbf{0.412}$_{\pm 0.007}$}   & \multicolumn{1}{c}{\textbf{0.142}$_{\pm 0.010}$}  & \multicolumn{1}{c}{\textbf{0.309}$_{\pm 0.009}$} & \textbf{15.89} & \textbf{1.7}                                                          & \textbf{34.12$_{\pm 1.98}$}                           & \textbf{97.88$_{\pm 1.89}$ }                          & \textbf{27.45$_{\pm 0.19}$} & \textbf{89.23$_{\pm 1.54}$}                      & \textbf{1.8}                                                          & \textbf{96.6}                                           \\ \hline
\end{tabular}}
\caption{The ablation study of the pre-training datasets. MRI-CT: Brain tumor MRI and CT scan dataset~\cite{brainctmri}. } 
	\label{abalation_data}
\end{table*}

\section{More Comparison with Multi-modal Generative Model}
\label{comparionwithmulti}
\begin{figure*}[h]
\centering
\includegraphics[width=1\linewidth]{a_mrict.pdf}
\caption{More generative samples of MRI synthesis tasks by our model and advanced text-to-image generative works CoDi~\cite{tang2023codi}, BIND~\cite{girdhar2023imagebind}, and VD~\cite{xu2023versatile}.}
\label{a_mrict}
\end{figure*}

\begin{figure*}[h]
\centering
\includegraphics[width=1\linewidth]{a_text2image.pdf}
\caption{More generative samples of medical text-to-image tasks by our model and advanced text-to-image generative works.}
\label{a_text2image}
\end{figure*}
We compare more generative samples with the advanced multi-modal generative model in Table~\ref{multi-modal} and ~\ref{a+text2image}, Fig.~\ref{a_mrict}. 
As depicted in Table~\ref{multi-modal}, we not only assess the performance of existing state-of-the-art (SOTA) multimodal generative models trained on their original extensively pre-trained data but also compare their outcomes when fine-tuned on our consistent medical pre-trained data. In-depth experimental comparisons suggest that, in contrast to these current SOTA models, our model not only shows a substantial edge in various generation tasks but also, under conditions with relatively limited training resources, proves its superiority in medical downstream tasks. It produces medical images of superior quality in terms of detail and reduced artifact levels, courtesy of the proposed medical visual invariance and cross-guided diffusion.

Besides, Table~\ref{a+text2image} presents the test results of our model and the state-of-the-art (SOTA) text-to-image generation models on three medical image generation datasets (ChestXray14~\cite{wang2017chestx}, ACDC~\cite{bernard2018deepACDC}, and SLIVER~\cite{heimann2009comparisonsliver} datasets), demonstrating the superior cross-modal generation performance of our model in text-to-image tasks.

\begin{table*}[h]
	\centering
	%\resizebox{8cm}{
	\scalebox{1}{% Please add the following required packages to your document preamble:
% \usepackage{multirow}
% Please add the following required packages to your document preamble:
% \usepackage{multirow}\
\small
	\setlength{\tabcolsep}{1pt}
	
%\begin{tabular}{lcccccccccccc}
\begin{tabular}{llllllllllll}
\hline
\multirow{2}{*}{Methods}             & \multicolumn{1}{c}{\multirow{2}{*}{\begin{tabular}[c]{@{}c@{}}Pre-train \\ Datasets\end{tabular}}} & \multicolumn{1}{c}{\multirow{2}{*}{\begin{tabular}[c]{@{}c@{}}Pre-train \\ samples\end{tabular}}} & \multicolumn{3}{c}{MIMIC-CXR}                                                          & \multicolumn{1}{c}{ACDC}   & MIMIC-CXR     & \multicolumn{2}{c}{BraTS}       & \multicolumn{2}{c}{Pelvic}      \\ \cline{4-12} 
                                     & \multicolumn{1}{c}{}                                                                               & \multicolumn{1}{c}{}                                                                              & \multicolumn{1}{c}{BLEU-1} & \multicolumn{1}{c}{BLEU-4} & \multicolumn{1}{c}{ROUGE\_L} & \multicolumn{1}{c}{Fid(↓)} & Fid           & PSNR           & SSIM           & PSNR           & SSIM           \\ \hline
\multirow{2}{*}{VD~\cite{xu2023versatile}} & original                                                                                           & 700M                                                                                              & 0.356$_{\pm 0.008}$                      & 0.008$_{\pm 0.009}$                      & 0.254$_{\pm 0.006}$                        & 30.12                      & 12.7          & 28.97$_{\pm 2.12}$          & 78.45$_{\pm 2.33}$          & 17.87$_{\pm 0.98}$          & 71.43$_{\pm 1.34}$          \\
                                     & \textbf{M+M+MC}                                                                              & 598K                                                                                              & \textbf{0.368}$_{\pm 0.010}$             & \textbf{0.112}$_{\pm 0.008}$             & \textbf{0.262}$_{\pm 0.006}$               & \textbf{26.67}             & \textbf{9.8}  & \textbf{29.88}$_{\pm 2.13}$ & \textbf{80.12}$_{\pm 2.54}$ & \textbf{19.21}$_{\pm 1.12}$ & \textbf{75.67}$_{\pm 1.18}$ \\\cline{2-12} 
\multirow{2}{*}{BIND~\cite{girdhar2023imagebind}}           & original                                                                                           & 2270K                                                                                             & 0.362$_{\pm 0.006}$                      & 0.101$_{\pm 0.009}$                      & 0.259$_{\pm 0.011}$                        & 32.14                      & 14.6           & 27.66$_{\pm 1.45}$          & 71.12$_{\pm 1.87}$          & 15.43$_{\pm 1.13}$          & 65.38$_{\pm 1.88}$     \\
                                     & \textbf{M+M+MC}                                                                              & 598K                                                                                              & \textbf{0.373}$_{\pm 0.005}$             & \textbf{0.109}$_{\pm 0.011}$             & \textbf{0.265}$_{\pm 0.007}$               & \textbf{28.34}             & \textbf{11.2} & \textbf{28.34}$_{\pm 2.22}$ & \textbf{75.34}$_{\pm 2.32}$ & \textbf{18.78}$_{\pm 1.05}$ & \textbf{69.23}$_{\pm 1.97}$ \\\cline{2-12} 
\multirow{2}{*}{CoDi~\cite{tang2023codi}}                & original                                                                                           & 512M                                                                                              & 0.369$_{\pm 0.006}$                      & 0.106$_{\pm 0.011}$                      & 0.266$_{\pm 0.005}$                        & 25.12                      & 10.9           & 29.12$_{\pm 2.11}$          & 80.68$_{\pm 1.86}$          & 19.12$_{\pm 0.88}$          & 73.23$_{\pm 1.22}$     \\
                                     & \textbf{M+M+MC}                                                                              & 598K                                                                                              & \textbf{0.381}$_{\pm 0.008}$             & \textbf{0.119}$_{\pm 0.009}$             & \textbf{0.273}$_{\pm 0.010}$               & \textbf{22.32}             & \textbf{7.8}  & \textbf{30.78}$_{\pm 2.45}$ & \textbf{84.44}$_{\pm 2.01}$ & \textbf{22.32}$_{\pm 1.43}$ & \textbf{78.86}$_{\pm 1.89}$ \\ \hline
\multicolumn{1}{l}{\textbf{Ours}}    & \textbf{M+M+MC}                                                                              & \textbf{598K}                                                                                     & \multicolumn{1}{c}{\textbf{0.412}$_{\pm 0.007}$}  & \multicolumn{1}{c}{\textbf{0.142}$_{\pm 0.010}$}  & \multicolumn{1}{c}{\textbf{0.309}$_{\pm 0.009}$}    & \multicolumn{1}{c}{\textbf{15.89}}  & \textbf{2.7}  & \textbf{34.12$_{\pm 1.98}$}                           & \textbf{97.88$_{\pm 1.89}$ }                          & \textbf{27.45$_{\pm 0.19}$} & \textbf{89.23$_{\pm 1.54}$} \\ \hline
\end{tabular}}
\caption{The comparison between MedM2G and advanced general multi-modal generative models. M+M+MC: Pre-training datasets of MIMIC-CXR, MedICat and Brain tumor MRI and CT scan.  } 
	\label{multi-modal}
\end{table*}
\begin{table*}[h]
	\centering
	%\resizebox{8cm}{
	\scalebox{1}{% Please add the following required packages to your document preamble:
% \usepackage{multirow}
% Please add the following required packages to your document preamble:
% \usepackage{multirow}\
\small
	\setlength{\tabcolsep}{10pt}
	
%\begin{tabular}{lcccccccccccc}
\begin{tabular}{lccc}
\hline
\multirow{2}{*}{Text-to-Image Method} & \multicolumn{3}{c}{Dataset Fid(↓)}             \\ \cline{2-4} 
                                      & ChestXray14   & ACDC           & SLIVER07      \\ \hline
Stable Diffusion-1.4~\cite{rombach2022highLDM}                & 20.13         & 35.32          & 38.76         \\
CogView~\cite{ding2021cogview}                               & 16.45         & 31.23          & 30.17         \\
Versatile Diffusion~\cite{xu2023versatile}                   & 11.43         & 26.67          & 24.39         \\
LDM~\cite{rombach2022highLDM}                                   & 10.33         & 26.02          & 21.72         \\
CoDi~\cite{rombach2022highLDM}                                  & 8.68          & 22.32          & 15.21         \\
Make-a-Scene~\cite{gafni2022makeasence}                          & 5.33          & 21.17          & 10.78         \\
GLIDE~\cite{nichol2021glide}                                 & 2.89          & 20.19          & 8.45          \\ \hline
Ours                                  & \textbf{1.84} & \textbf{15.89} & \textbf{6.89} \\ \hline
\end{tabular}}
\caption{The comparison between MedM2G and advanced general text-to-image models across ChestXray, ACDC, and SLIVER07 datasets.} 
	\label{a+text2image}
\end{table*}
\section{More computation Costs of Different Training Settings}
\label{sec:computation}
We provide more detailed computation costs of different training settings in Table ~\ref{computation}. We separately computed the pretraining time and the added model parameters for the three pretraining tasks in Table ~\ref{a_pre-train_tasks} and each multi-flow configuration. 
The computation results demonstrate the superior efficiency of our model. Benefiting from the proposed central alignment strategy, our model can achieve the unification of multiple medical modalities through multi-flow training, with a linear increase in computing cost, avoiding significant computational resource consumption like others.

\begin{table*}[h]
	\centering
	%\resizebox{8cm}{
	\scalebox{1}{% Please add the following required packages to your document preamble:
% \usepackage{multirow}
% Please add the following required packages to your document preamble:
% \usepackage{multirow}\
\small
	\setlength{\tabcolsep}{20pt}
	
%\begin{tabular}{lcccccccccccc}
\begin{tabular}{lccc}
\hline
\multicolumn{2}{c}{\multirow{2}{*}{Training Settings}} & \begin{tabular}[c]{@{}l@{}}Pre-training time\\ /epoch\end{tabular} & \begin{tabular}[c]{@{}l@{}}Add\\ Parameter\end{tabular} \\
\multicolumn{2}{c}{}                                   & /h                                                                 & /M                                                      \\ \hline
\multirow{4}{*}{Task1}          & Text→X-ray           & 0.2                                                                & 12.1                                                    \\
                                & X-ray→Text           & 0.2                                                                & 11.7                                                    \\
                                & Contrastive          & 0.5                                                                & 16.8                                                    \\
                                & Total                & 0.8                                                                & 33.8                                                    \\ \hline
\multirow{4}{*}{Task2}          & Text→CT              & 0.2                                                                & 13.2                                                    \\
                                & CT→Text              & 0.2                                                                & 11.9                                                    \\
                                & Contrastive          & 0.5                                                                & 18.6                                                    \\
                                & Total                & 0.7                                                                & 38.4                                                    \\ \hline
\multirow{4}{*}{Task3}          & CT→MRI               & 0.3                                                                & 19.8                                                    \\
                                & MRI→CT               & 0.3                                                                & 18.7                                                    \\
                                & Contrastive          & 0.4                                                                & 25.4                                                    \\
                                & Total                & 0.7                                                                & 41.2                                                    \\ \hline
\multicolumn{2}{c}{Single-flow(Task1)}                 & 0.8                                                                & 33.8                                                    \\
\multicolumn{2}{c}{Two-flow(Tasks1+2)}                 & 1.4                                                                & 55.9                                                    \\
\multicolumn{2}{c}{Three-flow(Task1+2+3)}              & 1.8                                                                & 96.6                                                    \\ \hline
\end{tabular}}
\caption{The computation costs of different training settings, including the pre-training tasks and the multi-flow strategies. } 
	\label{computation}
\end{table*}

\begin{table*}[h]
	\centering
	%\resizebox{8cm}{
	\scalebox{1}{% Please add the following required packages to your document preamble:
% \usepackage{multirow}
% Please add the following required packages to your document preamble:
% \usepackage{multirow}\
\small
	\setlength{\tabcolsep}{15pt}
	
%\begin{tabular}{lcccccccccccc}
\begin{tabular}{cccccc}
\hline
\multirow{2}{*}{Modality} & \multirow{2}{*}{Hyper} & \multicolumn{3}{c}{MIMIC-CXR}                    & ACDC           \\ \cline{3-6} 
                          &                        & BLEU-1         & BLEU-4         & ROUGE\_L       & Fid(↓)         \\ \hline
\multirow{4}{*}{Text}     & \textbf{2}             & \textbf{0.410}$_{\pm 0.009}$ & \textbf{0.141}$_{\pm 0.009}$ & \textbf{0.310}$_{\pm 0.011}$ & \textbf{15.86} \\
                          & 3                      & 0.407$_{\pm 0.007}$          & 0.135$_{\pm 0.010}$          & 0.303$_{\pm 0.011}$          & 16.67          \\
                          & 4                      & 0.405$_{\pm 0.008}$          & 0.133$_{\pm 0.011}$          & 0.306$_{\pm 0.009}$          & 16.45          \\
                          & 5                      & 0.404$_{\pm 0.009}$          & 0.132$_{\pm 0.010}$          & 0.304$_{\pm 0.008}$          & 16.16          \\ \hline
\multirow{4}{*}{CT}       & 2                      & 0.408$_{\pm 0.006}$          & 0.139$_{\pm 0.007}$          & 0.309$_{\pm 0.011}$          & 16.03          \\
                          & 3                      & 0.410$_{\pm 0.009}$          & 0.142$_{\pm 0.008}$          & 0.311$_{\pm 0.011}$          & 15.98          \\
                          & \textbf{4}             & \textbf{0.411}$_{\pm 0.011}$ & \textbf{0.144}$_{\pm 0.010}$ & \textbf{0.313}$_{\pm 0.009}$ & \textbf{15.91} \\
                          & 5                      & 0.408$_{\pm 0.008}$          & 0.143$_{\pm 0.006}$          & 0.312$_{\pm 0.010}$          & 15.99          \\ \hline
\multirow{4}{*}{MRI}      & 2                      & 0.405$_{\pm 0.006}$          & 0.138$_{\pm 0.008}$          & 0.309$_{\pm 0.007}$          & 16.13          \\
                          & 3                      & 0.408$_{\pm 0.009}$          & 0.141$_{\pm 0.011}$          & 0.311$_{\pm 0.009}$          & 16.02          \\
                          & \textbf{4}             & \textbf{0.412}$_{\pm 0.008}$ & \textbf{0.142}$_{\pm 0.008}$ & \textbf{0.312}$_{\pm 0.011}$ & \textbf{15.93} \\
                          & 5                      & 0.411$_{\pm 0.008}$          & 0.137$_{\pm 0.009}$          & 0.307$_{\pm 0.009}$          & 16.32          \\ \hline
\multirow{4}{*}{X-ray}    & 2                      & 0.412$_{\pm 0.012}$          & 0.141$_{\pm 0.014}$          & 0.308$_{\pm 0.011}$          & 16.28          \\
                          & 3                      & 0.415$_{\pm 0.011}$          & 0.143$_{\pm 0.011}$          & 0.308$_{\pm 0.009}$          & 16.07          \\
                          & \textbf{4}             & \textbf{0.416}$_{\pm 0.010}$ & \textbf{0.147}$_{\pm 0.009}$ & \textbf{0.315}$_{\pm 0.007}$ & \textbf{15.82} \\
                          & 5                      & 0.415$_{\pm 0.011}$          & 0.145$_{\pm 0.009}$          & 0.312$_{\pm 0.008}$          & 15.96          \\ \hline
\end{tabular}}
\caption{The influence of the depth of the four different UNet hyperparameters for text, CT, MRI, and X-ray modalities. } 
	\label{a_depth}
\end{table*}

\begin{table*}[h]
	\centering
	%\resizebox{8cm}{
	\scalebox{1}{% Please add the following required packages to your document preamble:
% \usepackage{multirow}
% Please add the following required packages to your document preamble:
% \usepackage{multirow}\
\small
	\setlength{\tabcolsep}{15pt}
	
%\begin{tabular}{lcccccccccccc}
\begin{tabular}{cccccc}
\hline
\multirow{2}{*}{Hyperparameter}  & \multirow{2}{*}{Settings} & \multicolumn{3}{c}{MIMIC-CXR}                    & ACDC           \\
                                 &                           & BLEU-1         & BLEU-4         & ROUGE\_L       & Fid(↓)         \\ \hline
\multirow{3}{*}{CA embed}        & 512                       & 0.405$_{\pm 0.008}$          & 0.139$_{\pm 0.010}$          & 0.306$_{\pm 0.007}$          & 16.32          \\
                                 & \textbf{768}              & \textbf{0.411}$_{\pm 0.009}$ & \textbf{0.144}$_{\pm 0.011}$ & \textbf{0.313}$_{\pm 0.012}$ & \textbf{15.91} \\
                                 & 1024                      & 0.408$_{\pm 0.008}$          & 0.141$_{\pm 0.007}$          & 0.309$_{\pm 0.009}$          & 16.12          \\ \hline
\multirow{3}{*}{Embedding layer} & 512                       & 0.406$_{\pm 0.010}$          & 0.141$_{\pm 0.009}$          & 0.311$_{\pm 0.008}$          & 15.99          \\
                                 & \textbf{768}              & \textbf{0.413}$_{\pm 0.013}$ & \textbf{0.143}$_{\pm 0.011}$ & \textbf{0.314}$_{\pm 0.008}$ & \textbf{15.89} \\
                                 & 1024                      & 0.409$_{\pm 0.007}$          & 0.138$_{\pm 0.006}$          & 0.312$_{\pm 0.008}$          & 16.04          \\ \hline
\multirow{2}{*}{CLIP scale size} & ViT-B                     & 0.412$_{\pm 0.011}$          & 0.142$_{\pm 0.009}$          & 0.312$_{\pm 0.010}$          & 15.93          \\
                                 & \textbf{Vit-L}            & \textbf{0.419}$_{\pm 0.008}$ & \textbf{0.151}$_{\pm 0.009}$ & \textbf{0.324}$_{\pm 0.011}$ & \textbf{14.89} \\ \hline
\end{tabular}}
\caption{The influence of the dimension of the cross-attention embedding and the embedding layer $\mathbb{F}_{emb}$, and the CLIP scale size of the prompt encoders. } 
	\label{a_hyper3}
\end{table*}

\begin{table*}[h]
	\centering
	%\resizebox{8cm}{
	\scalebox{1}{% Please add the following required packages to your document preamble:
% \usepackage{multirow}
% Please add the following required packages to your document preamble:
% \usepackage{multirow}\
\small
	\setlength{\tabcolsep}{20pt}
	
%\begin{tabular}{lcccccccccccc}
\begin{tabular}{lccc}
\hline
Hyperparameter    & \multicolumn{3}{c}{Dataset Fid(↓)}                                                                         \\ \hline
$\lambda_1$             & ChestXray14                       & \multicolumn{1}{c}{ACDC}           & \multicolumn{1}{c}{SLIVER07}      \\ \hline
5e-04          & \multicolumn{1}{c}{2.89}          & 16.78                              & 7.32                              \\
\textbf{5e-03}  & \multicolumn{1}{c}{\textbf{1.84}}                     & \multicolumn{1}{c}{\textbf{15.89}} & \multicolumn{1}{c}{\textbf{6.89}} \\
1e-03     & {{1.99}} & {16.12}                     &{7.02}  \\ 
1e-02     & {{2.13}} & {16.34}                     &{7.11}   \\\hline
\end{tabular}}
\caption{The influence of the non-negative balancing hyperparameter $\lambda_1$ in Eq. 4. } 
	\label{a_lanma}
\end{table*}

\section{Influence of Hyperparameters}
\label{influncence}
As shown in Table~\ref{a_depth}, \ref{a_hyper3} and \ref{a_lanma}, we demonstrate the influence of the various hyperparameters, including the depth of the UNet, the cross-attention embedding dimensions in the UNet, the dimension of the embedding layer $\mathbb{F}_{emb}$ in Section $3.4$, the scaling size of the CLIP prompt encoder for alignment, and the balancing hyperparameter $\lambda_1$ in Eq. 4.

\noindent\textbf{UNet Depth} In Table~\ref{a_depth}, 
we separately investigate the influence of the depth of the UNet network on the experimental results for the four modalities on the MIMIC-CXR~\cite{johnson2019mimic} and ACDC~\cite{bernard2018deepACDC} datasets. We set the depth to be $2-5$ layers, where the text UNet achieved the best performance at a depth of $2$, while CT, MRI, and X-ray all performed best when the depth was set to 4.

\noindent\textbf{Cross-attention Embedding} 
In Table~\ref{a_hyper3}, we investigate the impact of the cross-attention dimension in UNet. We conduct experiments with three settings for the embedding dimension of cross-attention: $512$, $768$, and $1024$. 
It is important to note that, to align the four modalities (Text, CT, MRI, X-ray), the embedding dimension of UNET is uniformly set for all modalities. The results indicate that the optimal performance is achieved when the embedding dimension of cross-attention is set to $768$.

\noindent\textbf{Dimension of Embedding Layer} In Table~\ref{a_hyper3}, 
we vary the dimension of the embedding layer $\mathbb{F}_{emb}$ in Section $3.4$ with three settings. The best performance on downstream tasks is achieved when the encoding dimension for all four modalities is set to $768$.

\noindent\textbf{CLIP Scale Size} As shown in Table~\ref{a_hyper3}, 
we pre-train the prompt encoder of four modalities with the ViT-Base, ViT-Large, and ViT-Huge settings. Our results demonstrate that the deeper and larger ViT model provides stronger improvements on the corresponding fine-tuning datasets. In our paper, to maintain the same settings as other models for fair comparison, we adopt the results of ViT-Base for comparison with other state-of-the-art models.

\noindent\textbf{Non-negative Balancing Hyperparameter} In Table~\ref{a_lanma}, we explore the influence of the non-negative balancing hyperparameter $\lambda_1$ in Eq. 4 across three medical image generation datasets ChestXray~\cite{wang2017chestx}, ACDC~\cite{bernard2018deepACDC}, and SLIVER07~\cite{heimann2009comparisonsliver}. We ran the experiment settings from $5e-4$ to $1e-2$ and found the best results for $\lambda_1=5e-3$, which is the same as the Barlow Twins~\cite{zbontar2021barlow}.
